# Supplementary material for: Distillation of Diffusion Features for Semantic Correspondence
Source: arXiv:2412.03512 source file (2024-12-04)
Supplement: Supplementary file 1 [file 5_appendix.tex]

\begin{table}[H]
\centering
\resizebox{\columnwidth}{!}{%
\begin{tabular}{lcccc}
\toprule
\textbf{Model} & \begin{tabular}{c} \textbf{SPair-71K} \\ \textbf{PCK@0.1} \\ \textbf{(img/bbox)} \end{tabular} & \begin{tabular}{c} \textbf{PF-WILLOW} \\ \textbf{PCK@0.1} \\ \textbf{(img/bbox)} \end{tabular} & \begin{tabular}{c} \textbf{CUB-200} \\ \textbf{PCK@0.1} \\ \textbf{(img/bbox)} \end{tabular} & \begin{tabular}{c} \textbf{Resolution} \\ \textbf{Timesteps} \\ \textbf{Layers} \\ \textbf{Prompt} \end{tabular} \\
\midrule
SD1.5 & $66.11 / 56.24$ & $86.58 / 73.60$ & $90.58 / 79.18$ & \begin{tabular}{c}$(768, 768)$ \\ $\{201\}$ \\ $\{5\}$ \\ ``a photo of a [category]" \end{tabular} \\
\midrule
SD2.1 & \underline{$65.29 / 57.87$} & $87.18 / 74.83$ & $88.63 / 78.23$ & \begin{tabular}{c}$(768, 768)$ \\ $\{261\}$ \\ $\{8\}$ \\ ``a photo of a [category]" \end{tabular} \\
\midrule
SDXL Base & \begin{tabular}{c}$64.02 / 55.52$ \\ $65.64 / 57.87$\end{tabular} & \begin{tabular}{c}\underline{$88.37 / 76.49$} \\ $88.58 / 76.30$\end{tabular} & \begin{tabular}{c}$92.39 / 84.20$ \\ $92.41 / 84.20$\end{tabular} & \begin{tabular}{c}$(768, 768)$ and $(1024, 1024)$ \\ $\{101\}$ and $\{201\}$ \\ $\{1\}$ \\ ``a photo of a [category]" \end{tabular} \\
\midrule
LCM-XL & \begin{tabular}{c}$62.9 / 54.5$ \\ $63.2 / 55.8$\end{tabular} & \begin{tabular}{c}$86.52 / 73.81$ \\ $85.86 / 74.04$\end{tabular} & \begin{tabular}{c}\underline{$92.59 / 84.40$} \\ $92.70 / 84.91$\end{tabular} & \begin{tabular}{c}$(768, 768)$ and $(1024, 1024)$ \\ $\{64\}$ \\ $\{1\}$ \\ ``a photo of a [category]" \end{tabular} \\
\midrule
SDXL Turbo & \begin{tabular}{c}\textbf{$67.26 / 58.54$} \\ $67.4 / 59.5$\end{tabular} & \begin{tabular}{c}\textbf{$89.59 / 77.76$} \\ $88.48 / 76.44$\end{tabular} & \begin{tabular}{c}\textbf{$93.54 / 85.57$} \\ $93.35 / 85.72$\end{tabular} & \begin{tabular}{c}$(768, 768)$ and $(1024, 1024)$ \\ $\{101\}$ \\ $\{1\}$ \\ ``a photo of a [category]" \end{tabular} \\
\bottomrule
\end{tabular}
}
\label{tbl:diff}
\caption{The performance of different diffusion-based models.}
\end{table}

\begin{table}[H]
\centering
\resizebox{\columnwidth}{!}{%
\begin{tabular}{lcccc}
\toprule
\textbf{Model} & \begin{tabular}{c} \textbf{SPair-71K} \\ \textbf{PCK@0.1} \\ \textbf{(img/bbox)} \end{tabular} & \begin{tabular}{c} \textbf{PF-WILLOW} \\ \textbf{PCK@0.1} \\ \textbf{(img/bbox)} \end{tabular} & \begin{tabular}{c} \textbf{CUB-200} \\ \textbf{PCK@0.1} \\ \textbf{(img/bbox)} \end{tabular} & \begin{tabular}{c} \textbf{Resolution} \\ \textbf{Layers} \end{tabular} \\
\midrule
DINOv1 (vits8) & $46.69 / 35.92$ & $61.66 / 47.99$ & $84.06 / 70.09$ & \begin{tabular}{c}$(224, 224)$ \\ Layer 9 \end{tabular} \\
\midrule
DINOv2 (vitb14) & \underline{$67.45 / 57.69$} & \textbf{$84.14 / 68.78$} & \underline{$94.54 / 85.90$} & \begin{tabular}{c}$(840, 840)$ \\ Layer 11 \end{tabular} \\
\midrule
DINOv2 (vitb14) \\ with registers & \textbf{$69.10 / 58.83$} & \underline{$83.07 / 67.38$} & \textbf{$94.61 / 85.90$} & \begin{tabular}{c}$(840, 840)$ \\ Layer 11 \end{tabular} \\
\midrule
CLIP \\ (ViT-L-14) & $47.05 / 37.05$ & $73.51 / 57.67$ & $82.31 / 67.86$ & \begin{tabular}{c}$(336, 336)$ \\ Layer 11 \end{tabular} \\
\midrule
MAE \\ (ViT-L-14) & $33.26 / 23.99$ & $73.04 / 56.54$ & $64.25 / 45.04$ & \begin{tabular}{c}$(224, 224)$ \\ Layer 26 \end{tabular} \\
\midrule
ZoeDepth & $12.8 / 6.63$ & $38.47 / 25.93$ & $22.90 / 9.75$ & \begin{tabular}{c}$(512, 384)$ \\ Layer 10 (BeiT) \end{tabular} \\
\midrule
I-JEPA \\ (ViT-H-16 448) & $51.88 / 44.78$ & $- / -$ & $- / -$ & \begin{tabular}{c}$(448, 448)$ \\ Layer 31 \end{tabular} \\
\bottomrule
\end{tabular}
}
\label{tbl:vit}
\caption{The performance of different ViT-based models.}
\end{table}

\begin{table}[H]
\centering
\resizebox{\columnwidth}{!}{%
\begin{tabular}{lcccc}
\toprule
\textbf{Model} & \begin{tabular}{c} \textbf{SPair-71K} \\ \textbf{PCK@0.1} \\ \textbf{(img/bbox)} \end{tabular} & \begin{tabular}{c} \textbf{PF-WILLOW} \\ \textbf{PCK@0.1} \\ \textbf{(img/bbox)} \end{tabular} & \begin{tabular}{c} \textbf{CUB-200} \\ \textbf{PCK@0.1} \\ \textbf{(img/bbox)} \end{tabular} & \begin{tabular}{c} \textbf{Resolution} \\ \textbf{Timesteps} \\ \textbf{Layers} \\ \textbf{Prompt} \end{tabular} \\
\midrule
SDXL Turbo + DINOv2 & $70.90 / 61.88$ & \textbf{$89.77 / 76.62$} & \underline{$94.89 / 86.45$} & \begin{tabular}{c}$[840, 840]$ \\ ADD: $\{1\}$, 101 \\ DINO: $\{11\}$ \\ ``a photo of a [category]" \end{tabular} \\
\midrule
SDXL Turbo + DINOv2\ & $71.21 / 62.79$ & $88.03 / 74.76$ & $94.22 / 85.81$ & \begin{tabular}{c}$[840, 840]$ \\ ADD: $\{1, 4, 7\}$, 101 \\ DINO: $\{11\}$ \\ ``a photo of a [category]" \end{tabular} \\
\midrule
SDXL Turbo + DINOv2 & \textbf{$71.77 / 63.29$} & \underline{$89.36 / 75.98$} & \textbf{$94.83 / 87.43$} & \begin{tabular}{c}$[980, 980]$ \\ ADD: $\{1\}$, 101 \\ DINO: $\{11\}$ \\ ``a photo of a [category]" \end{tabular} \\
\midrule
SD1.5 + DINOv2 & $71.57 / 62.03$ & $89.02 / 75.94$ & $94.43 / 85.27$ & \begin{tabular}{c}$[840, 840]$ \\ SD: $\{5\}$, 201 \\ DINO: $\{11\}$ \\ ``a photo of a [category]" \end{tabular} \\
\midrule
SD1.5 + DINOv2 & $71.38 / 62.08$ & $88.84 / 75.70$ & $94.24 / 85.69$ & \begin{tabular}{c}$[840, 840]$ \\ SD: $\{3, 7, 11\}$, 201 \\ DINO: $\{11\}$ \\ ``a photo of a [category]" \end{tabular} \\
\midrule
SD1.5 + DINOv2 \cite{zhang2023tale} & \begin{tabular}{c}\underline{$71.67 / 63.08$} \\ $(- / 62.9)$\end{tabular} & \begin{tabular}{c}$88.43 / 74.84$ \\ $(- / -)$\end{tabular} & \begin{tabular}{c}$94.55 / 86.25$ \\ $(- / -)$\end{tabular} & \begin{tabular}{c}$(960, 960)$ \\ SD: $\{3, 7, 11\}$, 100 \\ DINO: $\{11\}$ \\ ``a photo of a [category]" \end{tabular} \\
\bottomrule
\end{tabular}
}
\label{tbl:combinations}
\caption{The performance of different combinations of models and layers.}
\end{table}
