# Supplementary material for: Distillation of Diffusion Features for Semantic Correspondence
Source: arXiv:2412.03512 source file (2024-12-04)
Supplement: Supplementary file 2 [file supplementary.tex]

\documentclass{article}
\usepackage{graphicx}
\usepackage{booktabs}
\usepackage{float}
\usepackage{amsmath}
\usepackage[pagebackref,breaklinks,colorlinks]{hyperref}
\usepackage[a4paper, margin=1in]{geometry}
\usepackage{array}
\usepackage[table]{xcolor}

% Support for easy cross-referencing
\usepackage[capitalize]{cleveref}
\crefname{section}{Sec.}{Secs.}
\Crefname{section}{Section}{Sections}
\Crefname{table}{Table}{Tables}
\crefname{table}{Tab.}{Tabs.}

\title{Supplementary Material}
\date{}

\begin{document}

\maketitle

\input{supp_content}
\end{document}
